# Supplementary material for: Adaptive Text Recognition through Visual Matching
Source: arXiv:2009.06610 source file (2020-09-14)
Supplement: Supplementary file 1 [file test_unseenfont.txt.tex]

\item Aclonica.ttf
\item CherryCreamSoda.ttf
\item CherryCreamSoda-VTT.ttf
\item Chewy.ttf
\item Chewy-VTT.ttf
\item ComingSoon.ttf
\item ComingSoon-TTX.ttf
\item CraftyGirls.ttf
\item CraftyGirls-TTX.ttf
\item Crushed.ttf
\item DroidSans.ttf
\item DroidSansMono.ttf
\item DroidSerif.ttf
\item FontdinerSwanky.ttf
\item HomemadeApple.ttf
\item IrishGrover.ttf
\item IrishGrowler.ttf
\item JustAnotherHand.ttf
\item Kranky.ttf
\item LuckiestGuy.ttf
\item MaidenOrange.ttf
\item PermanentMarker.ttf
\item Redressed.ttf
\item Roboto-Black.ttf
\item Roboto-Medium.ttf
\item Roboto-Thin.ttf
\item RobotoSlab-Thin.ttf
\item RockSalt.ttf
\item Schoolbell.ttf
\item Slackey.ttf
\item SpecialElite.ttf
\item Sunshiney.ttf
\item Ultra.ttf
\item WalterTurncoat-VTT.ttf
\item WalterTurncoat.ttf
\item AdventPro-Medium.ttf
\item AdventPro-Thin.ttf
\item Alegreya-Black.ttf
\item AlegreyaSans-Black.ttf
\item AlegreyaSans-Medium.ttf
\item AlegreyaSans-Thin.ttf
\item AlegreyaSansSC-Black.ttf
\item AlegreyaSansSC-Medium.ttf
\item AlegreyaSansSC-Thin.ttf
\item AlegreyaSC-Black.ttf
\item Amiri-Slanted.ttf
\item Andika-R.ttf
\item AnnieUseYourTelescope.ttf
\item Anton.ttf
\item Anton-VTT.ttf
\item ArchitectsDaughter.ttf
\item Asset.ttf
\item Bangers.ttf
\item Bevan.ttf
\item Bevan.ttf
\item Bevan\_ik.ttf
\item Bevan\_VTT - Copy.ttf
\item Bevan\_VTT.ttf
\item Bevan\_VTT2.ttf
\item BevanFLAB.ttf
\item BigshotOne.ttf
\item Cabin-Medium.ttf
\item CabinCondensed-Medium.ttf
\item Candal.ttf
\item Cantarell-Oblique.ttf
\item CarterOne.ttf
\item Cedarville-Cursive.ttf
\item Chivo-Black.ttf
\item Chivo-Black-VTT.ttf
\item Cinzel-Black.ttf
\item CinzelDecorative-Black.ttf
\item Coda-Heavy.ttf
\item CodaCaption-Heavy.ttf
\item Coustard-Black.ttf
\item CoveredByYourGrace.ttf
\item CrimsonText-Roman.ttf
\item cwTeXFangSong.ttf
\item cwTeXHei-ofl.ttf
\item cwTeXHei.ttf
\item cwTeXKai-ofl.ttf
\item cwTeXKai.ttf
\item cwTeXMing-ofl.ttf
\item cwTeXMing.ttf
\item cwTeXYen-ofl.ttf
\item cwTeXYen.ttf
\item DawningofaNewDay.ttf
\item DidactGothic.ttf
\item Dosis-Medium.ttf
\item Elsie-Black.ttf
\item ElsieSwashCaps-Black.ttf
\item Exo-Black.ttf
\item Exo-Medium.ttf
\item Exo-Thin.ttf
\item Exo2-Black.ttf
\item Exo2-Medium.ttf
\item Exo2-Thin.ttf
\item ExpletusSans-Medium.ttf
\item FiraSans-Medium.ttf
\item FrancoisOne.ttf
\item GenBasB.ttf
\item GenBasBI.ttf
\item GenBasI.ttf
\item GenBasR.ttf
\item GenBkBasB.ttf
\item GenBkBasBI.ttf
\item GenBkBasI.ttf
\item GenBkBasR.ttf
\item Geo-Oblique.ttf
\item GFSDidot.ttf
\item GFSNeohellenic.ttf
\item GFSNeohellenic.ttf
\item GiveYouGlory.ttf
\item GloriaHallelujah.ttf
\item GoblinOne.ttf
\item GoudyBookletter1911.ttf
\item GravitasOne.ttf
\item BM-HANNA.ttf
\item Hanuman.ttf
\item Hanumanb.ttf
\item HoltwoodOneSC.ttf
\item IMFeDPit28P.ttf
\item IMFeDPrm28P.ttf
\item IMFeDPsc28P.ttf
\item IMFePIit28P.ttf
\item IMFePIrm28P.ttf
\item IMFePIsc28P.ttf
\item IMFeENit28P.ttf
\item IMFeENrm28P.ttf
\item IMFeENsc28P.ttf
\item IMFeFCit28P.ttf
\item IMFeFCrm28P.ttf
\item IMFeFCsc28P.ttf
\item IMFeGPit28P.ttf
\item IMFeGPrm28P.ttf
\item IMFeGPsc28P.ttf
\item IndieFlower.ttf
\item Jomolhari-alpha3c-0605331.ttf
\item JosefinSans-Thin.ttf
\item JosefinSlab-Thin.ttf
\item Jura-Medium.ttf
\item JustMeAgainDownHere.ttf
\item Kristi.ttf
\item LaBelleAurore.ttf
\item LateefRegOT.ttf
\item Lato-Black.ttf
\item Lato-Hairline.ttf
\item LeagueScript.ttf
\item Lobster.ttf
\item Lobster-Cyrillic-TTF.ttf
\item LovedbytheKing.ttf
\item LoveYaLikeASister.ttf
\item MavenPro-Black.ttf
\item MavenPro-Medium.ttf
\item MavenPro-Black-VTT.ttf
\item MavenPro-Medium-VTT.ttf
\item Meddon.ttf
\item MedievalSharp.ttf
\item Megrim.ttf
\item Merriweather-Black.ttf
\item Metrophobic.ttf
\item Miama.ttf
\item Michroma.ttf
\item Monofett.ttf
\item Neucha.ttf
\item Neucha-hints.ttf
\item Nobile-Medium.ttf
\item NothingYouCouldDo.ttf
\item NovaCut.ttf
\item NovaFlat.ttf
\item NovaMono.ttf
\item NovaOval.ttf
\item NovaRound.ttf
\item NovaScript.ttf
\item NovaSlim.ttf
\item NovaSquare.ttf
\item OFLGoudyStMTT.ttf
\item Orbitron-Black.ttf
\item Orbitron-Medium.ttf
\item Overlock-Black.ttf
\item OvertheRainbow.ttf
\item Pacifico.ttf
\item padauk\_src.ttf
\item padaukbook\_src.ttf
\item PassionOne-Black.ttf
\item PaytoneOne.ttf
\item Pecita.ttf
\item PlayfairDisplay-Black.ttf
\item PlayfairDisplaySC-Black.ttf
\item PollerOne.ttf
\item PTM55FT.ttf
\item PTF55F.ttf
\item PTF56F.ttf
\item PTF75F.ttf
\item PTF76F.ttf
\item PTZ55F.ttf
\item PTZ56F.ttf
\item Raleway-Heavy.ttf
\item Raleway-Medium.ttf
\item Raleway-Thin.ttf
\item ReenieBeanie.ttf
\item ReenieBeanie-VTT.ttf
\item Ruda-Black.ttf
\item RuslanDisplay.ttf
\item SansitaOne.ttf
\item ScheherazadeRegOT.ttf
\item SeoulHangang-Medium.ttf
\item SeoulHangang.ttf
\item SeoulHangangB.ttf
\item SeoulHangangCondensed-Medium.ttf
\item SeoulHangang.ttf
\item SeoulHangangB.ttf
\item SeoulNamsan-Medium.ttf
\item SeoulNamsan.ttf
\item SeoulNamsanB.ttf
\item SeoulNamsanCondensed-Black.ttf
\item SeoulNamsanCondensed-Medium.ttf
\item SeoulNamsan.ttf
\item SeoulNamsanB.ttf
\item SigmarOne.ttf
\item Simonetta-Black.ttf
\item SixCaps.ttf
\item Snippet.ttf
\item SourceCodePro-Black.ttf
\item SourceCodePro-Medium.ttf
\item SourceSansPro-Black.ttf
\item SueEllenFrancisco.ttf
\item SwankyandMooMoo.ttf
\item TerminalDosis-Medium.ttf
\item Thabit-Oblique.ttf
\item Thabit.ttf
\item TheGirlNextDoor.ttf
\item Tienne-Heavy.ttf
\item TitilliumWeb-Black.ttf
\item UnifrakturMaguntia-Book.ttf
\item WaitingfortheSunrise.ttf
\item WireOne.ttf
\item Zeyada.ttf
\item Ubuntu-B-hinting.ttf
\item Ubuntu-BI-hinting.ttf
\item Ubuntu-C-hinting.ttf
\item Ubuntu-L-hinting.ttf
\item Ubuntu-LI-hinting.ttf
\item Ubuntu-M-hinting.ttf
\item Ubuntu-MI-hinting.ttf
\item Ubuntu-R-hinting.ttf
\item Ubuntu-RI-hinting.ttf
\item Ubuntu-Medium.ttf
\item UbuntuMono-B-hinting.ttf
\item UbuntuMono-BI-hinting.ttf
\item UbuntuMono-R-hinting.ttf
\item UbuntuMono-RI-hinting.ttf
