# Supplementary material for: Adaptive Text Recognition through Visual Matching
Source: arXiv:2009.06610 source file (2020-09-14)
Supplement: Supplementary file 2 [file train_fontlist_Light.txt.tex]

\item OpenSans-Light.ttf
\item Roboto-Light.ttf
\item RobotoCondensed-Light.ttf
\item RobotoSlab-Light.ttf
\item AdventPro-Light.ttf
\item AlegreyaSans-Light.ttf
\item AlegreyaSansSC-Light.ttf
\item Antonio-Light.ttf
\item AveriaLibre-Light.ttf
\item AveriaSerifLibre-Light.ttf
\item BenchNine-Light.ttf
\item Buda-Light.ttf
\item Codystar-Light.ttf
\item Comfortaa-Light.ttf
\item Dosis-Light.ttf
\item Exo-Light.ttf
\item Exo2-Light.ttf
\item FiraSans-Light.ttf
\item Flamenco-Light.ttf
\item Jura-Light.ttf
\item Kreon-Light.ttf
\item Lato-Light.ttf
\item Merriweather-Light.ttf
\item MerriweatherSans-Light.ttf
\item Muli-Light.ttf
\item Neuton-Light.ttf
\item Oswald-Light.ttf
\item Oxygen-Light.ttf
\item Raleway-Light.ttf
\item Rokkitt-Light.ttf
\item Sansation-Light.ttf
\item SeoulHangang-Light.ttf
\item SeoulHangangCondensed-Light.ttf
\item SeoulNamsan-Light.ttf
\item SeoulNamsanCondensed-Light.ttf
\item Signika-Light.ttf
\item SignikaNegative-Light.ttf
\item SourceCodePro-Light.ttf
\item SourceSansPro-Light.ttf
\item Stoke-Light.ttf
\item TitilliumWeb-Light.ttf
\item Tulpen-Light.ttf
\item YanoneKaffeesatz-Light.ttf
\item Ubuntu-Light.ttf
\item YanoneKaffeesatz-ExtraLight.ttf
\item Exo2-ExtraLight.ttf
\item Neuton-ExtraLight.ttf
\item Raleway-ExtraLight.ttf
\item TitilliumWeb-ExtraLight.ttf
\item YanoneKaffeesatz-ExtraLight.ttf
