# Supplementary material for: Adaptive Text Recognition through Visual Matching
Source: arXiv:2009.06610 source file (2020-09-14)
Supplement: Supplementary file 3 [file train_fontlist_italic.txt.tex]

\item NotoSans-Italic.ttf
\item NotoSansUI-Italic.ttf
\item OpenSans-Italic.ttf
\item OpenSansHebrew-Italic.ttf
\item Amaranth-Italic.ttf
\item Andada-Italic.ttf
\item AnonymousPro-Italic.ttf
\item Caudex-Italic.ttf
\item ChangaOne-Italic.ttf
\item ChauPhilomeneOne-Italic.ttf
\item Exo-Italic.ttf
\item FiraSans-Italic.ttf
\item Fondamento-Italic.ttf
\item IstokWeb-Italic.ttf
\item JosefinSans-Italic.ttf
\item JosefinSlab-Italic.ttf
\item Karla-Italic.ttf
\item Lekton-Italic.ttf
\item Lora-Italic.ttf
\item Muli-Italic.ttf
\item Neuton-Italic.ttf
\item NoticiaText-Italic.ttf
\item Oregano-Italic.ttf
\item Overlock-Italic.ttf
\item PlayfairDisplay-Italic.ttf
\item QuattrocentoSans-Italic.ttf
\item Quicksand-Italic.ttf
\item Radley-Italic.ttf
\item Sanchez-Italic.ttf
\item Sarabun-Italic.ttf
\item Sedan-Italic.ttf
\item SourceSansPro-Italic.ttf
\item Trochut-Italic.ttf
\item Vollkorn-Italic.ttf
\item Chivo-BlackItalic.ttf
\item Exo-BlackItalic.ttf
\item Exo2-BlackItalic.ttf
\item AlegreyaSans-MediumItalic.ttf
\item AlegreyaSansSC-MediumItalic.ttf
\item Share-BoldItalic.ttf
\item TitilliumWeb-SemiBoldItalic.ttf
\item Volkhov-BoldItalic.ttf
\item AlegreyaSansSC-LightItalic.ttf
\item AveriaLibre-LightItalic.ttf
\item AveriaSansLibre-LightItalic.ttf
\item AveriaSerifLibre-LightItalic.ttf
\item CrimsonText-BoldItalic.ttf
\item CrimsonText-SemiboldItalic.ttf
\item Cuprum-BoldItalic.ttf
\item Exo-ExtraBoldItalic.ttf
