# Supplementary material for: Adaptive Text Recognition through Visual Matching
Source: arXiv:2009.06610 source file (2020-09-14)
Supplement: Supplementary file 4 [file train_fontlist_regular.txt.tex]

\item Arimo-Regular.ttf
\item Calligraffitti-Regular.ttf
\item Cousine-Regular.ttf
\item MountainsofChristmas-Regular.ttf
\item NotoSans-Regular.ttf
\item RobotoCondensed-Regular.ttf
\item RobotoSlab-Regular.ttf
\item Rochester-Regular.ttf
\item Smokum-Regular.ttf
\item AllertaStencil-Regular.ttf
\item AveriaSansLibre-Regular.ttf
\item Balthazar-Regular.ttf
\item Basic-Regular.ttf
\item Baumans-Regular.ttf
\item Belgrano-Regular.ttf
\item BenchNine-Regular.ttf
\item BrunoAceSC-Regular.ttf
\item BubblegumSans-Regular.ttf
\item ButterflyKids-Regular.ttf
\item CabinSketch-Regular.ttf
\item Cambo-Regular.ttf
\item CantataOne-Regular.ttf
\item Clara-Regular.ttf
\item ClickerScript-Regular.ttf
\item Codystar-Regular.ttf
\item Comfortaa-Regular.ttf
\item ConcertOne-Regular.ttf
\item Condiment-Regular.ttf
\item Convergence-Regular.ttf
\item Cookie-Regular.ttf
\item Copse-Regular.ttf
\item DuruSans-Regular.ttf
\item Dynalight-Regular.ttf
\item Eater-Regular.ttf
\item EaterCaps-Regular.ttf
\item EBGaramond-Regular.ttf
\item Economica-Regular.ttf
\item EmblemaOne-Regular.ttf
\item Englebert-Regular.ttf
\item Jura-Regular.ttf
\item Kameron-Regular.ttf
\item KellySlab-Regular.ttf
\item KottaOne-Regular.ttf
\item KronaOne-Regular.ttf
\item Lancelot-Regular.ttf
\item Lato-Regular.ttf
\item Lekton-Regular.ttf
\item Lemon-Regular.ttf
\item UbuntuMono-Regular.ttf
