# Supplementary material for: Adaptive Text Recognition through Visual Matching
Source: arXiv:2009.06610 source file (2020-09-14)
Supplement: Supplementary file 5 [file train_fontlist_Bold.txt.tex]

\item Alef-Bold.ttf
\item Allan-Bold.ttf
\item AmaticSC-Bold.ttf
\item Amiri-Bold.ttf
\item Andada-Bold.ttf
\item Antonio-Bold.ttf
\item Comfortaa-Bold.ttf
\item Corben-Bold.ttf
\item DancingScript-Bold.ttf
\item Economica-Bold.ttf
\item FiraMono-Bold.ttf
\item Gorditas-Bold.ttf
\item Gudea-Bold.ttf
\item Inika-Bold.ttf
\item IstokWeb-Bold.ttf
\item JosefinSans-Bold.ttf
\item Judson-Bold.ttf
\item Kameron-Bold.ttf
\item Karla-Bold.ttf
\item Lekton-Bold.ttf
\item LibreCaslonText-Bold.ttf
\item Lora-Bold.ttf
\item Magra-Bold.ttf
\item Merienda-Bold.ttf
\item MerriweatherSans-Bold.ttf
\item Monda-Bold.ttf
\item MontserratSubrayada-Bold.ttf
\item NanumGothicCoding-Bold.ttf
\item NanumMyeongjo-Bold.ttf
\item PassionOne-Bold.ttf
\item Podkova-Bold.ttf
\item Puritan-Bold.ttf
\item Quattrocento-Bold.ttf
\item Raleway-Bold.ttf
\item Rokkitt-Bold.ttf
\item Rosario-Bold.ttf
\item Rufina-Bold.ttf
\item Scada-Bold.ttf
\item SeoulHangang-Bold.ttf
\item SeoulHangangCondensed-Bold.ttf
\item Share-Bold.ttf
\item SignikaNegative-Bold.ttf
\item Sintony-Bold.ttf
\item Skranji-Bold.ttf
\item SourceCodePro-Bold.ttf
\item Thabit-Bold.ttf
\item UnifrakturCook-Bold.ttf
\item YanoneKaffeesatz-Bold.ttf
\item Ubuntu-Bold.ttf
\item UbuntuMono-Bold.ttf
